# Supplementary material for: Signed, Sealed,... Confused: Exploring the Understandability and Severity of Policy Documents
Source: arXiv:2502.08743 source file (2025-02-12)
Supplement: Supplementary file 1 [file Supp-CaseBoxplots.tex]

\section{Per-Case Boxplots}

\FIXME{JED@SNS: What is going on with the content between here and "summary"? Which R\#-\# is it trying to resolve? My suspicion is that we want this in the supplement

@JED: Yes, these plots would be best to be included in the supplemental material.}
\begin{figure}
    \centering
    \includegraphics[width=\linewidth]{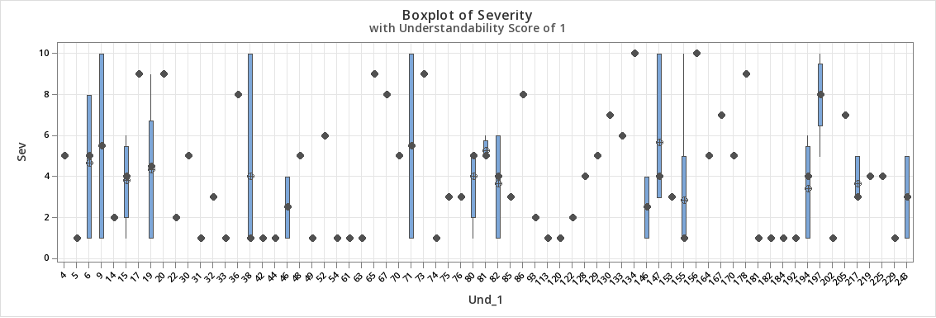}
    \caption{Enter Caption}
\end{figure}
In cases with an understandability score of 1, the wide spread of severity ratings, along with numerous outliers, suggests a lack of consensus on the impact of low clarity on severity judgments. While one might expect low understandability to correlate with high perceived severity due to confusion or ambiguity, the variability observed implies that participants’ severity ratings are influenced by other factors, such as their interpretation of the underlying context or their tolerance for ambiguity. This variability underscores the multifaceted nature of decision-making in the face of unclear information.

\begin{figure}
    \centering
    \includegraphics[width=\linewidth]{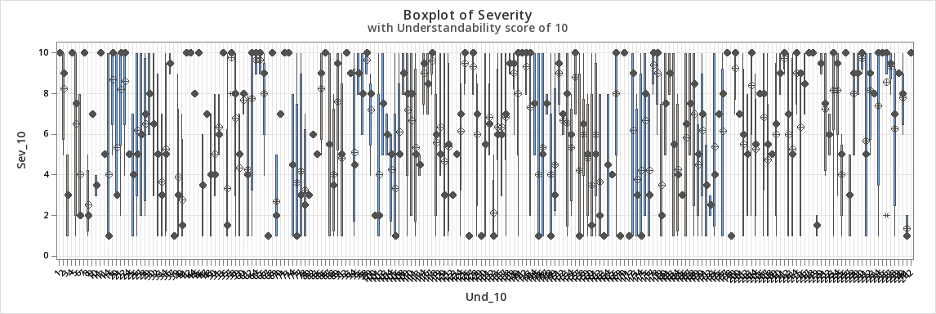}
    \caption{Enter Caption}
\end{figure}
The analysis of the boxplots reveals significant insights into the complex relationships between understandability and severity ratings. For cases with an understandability score of 10, the variability in severity ratings indicates that while high clarity is often associated with consistent severity evaluations, this is not universally true. The presence of outliers and wide interquartile ranges for some cases suggests that even when participants find content clear, their perceptions of its severity can vary, potentially due to differences in individual priorities, contextual interpretations, or subjective biases. This finding highlights that clarity alone does not uniformly mitigate the perception of severity.

\begin{figure}
    \centering
    \includegraphics[width=\linewidth]{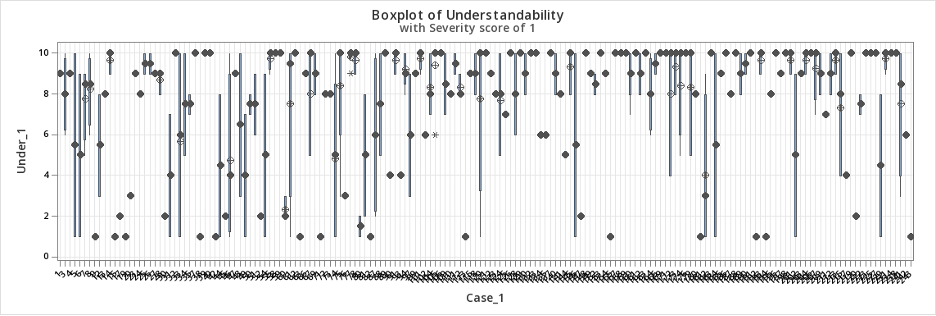}
    \caption{Enter Caption}
\end{figure}
For cases with a severity score of 1, the corresponding understandability ratings reveal diverse participant interpretations, with significant variability and outliers across cases. This suggests that even when a situation is deemed minimally severe, perceptions of its clarity can range widely. Such diversity may stem from differing levels of familiarity with the subject matter, contextual nuances, or individual cognitive approaches to understanding the content. This finding emphasizes that low severity does not guarantee consensus on understandability, highlighting the independent nature of these dimensions.
\begin{figure}
    \centering
    \includegraphics[width=\linewidth]{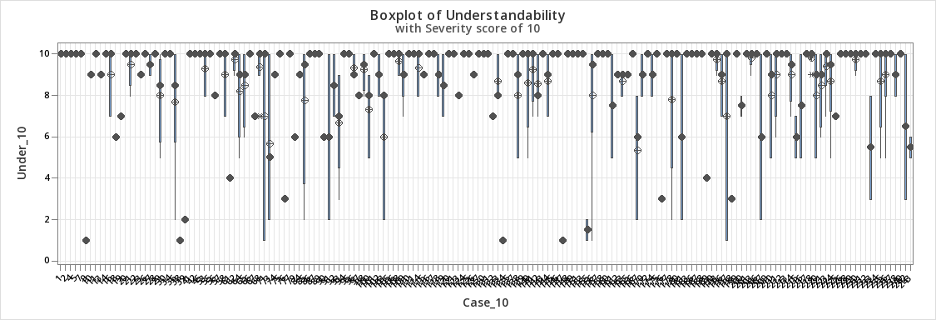}
    \caption{Enter Caption}
\end{figure}
Conversely, for cases with a severity score of 10, understandability ratings exhibit a tendency toward higher values, indicating that participants often find highly severe cases to be relatively clear. However, the presence of broad variability and outliers reveals that this is not a consistent pattern. Some participants rate such cases as less clear, suggesting that factors such as technical complexity, emotional impact, or the framing of information play roles in shaping perceptions of clarity even in the presence of high severity.

Overall, the findings indicate that understandability and severity are interrelated yet distinct dimensions, each shaped by a complex interplay of subjective, contextual, and content-specific factors. The variability and lack of strong linear correlation between the two dimensions highlight the need for nuanced frameworks that account for these influences when evaluating the relationship between clarity and perceived impact in different scenarios.
