# Supplementary material for: Signed, Sealed,... Confused: Exploring the Understandability and Severity of Policy Documents
Source: arXiv:2502.08743 source file (2025-02-12)
Supplement: Supplementary file 2 [file Supp-Organization.tex]

\section{Organization}

This repo consists of the following items:
\begin{enumerate}
\item Motivations:
    \begin{itemize}
        \item How motivated are you to read privacy policies before using an online service to make sure your information is safe?	

        Polarity: 1 means ‘Not motivated at all’ and 10 means ‘Extremely motivated’
        %JED: do we want to label the median?
        
        %(If 5, Scale: Not motivated, Slightly motivated, Moderately motivated, Highly motivated, Extremely motivated)
        \item How likely are you to invest time in understanding privacy policies to avoid potential privacy issues?
        
        Polarity: 1 means ‘Very unlikely’ and 10 means ‘Very likely’
        %JED: do we want to label the median?

        %(If 5, Scale: Very unlikely, Unlikely, Neutral, Likely, Very likely)
    \end{itemize}
\item Information Processing Style:
    \begin{itemize}
        %\item How much would you like detailed explanations over short summaries?
        % \item Which do you prefer between detailed explanations or short summaries?

        % Scale: Greatly prefer detailed explanations (1) - Greatly prefer short summaries (10)
        %JED: do you want them to take a stand?, would fewer items be better?

        % Scale: Prefer short summaries, Slightly prefer detailed explanations, Neutral, Prefer detailed explanations, Strongly prefer detailed explanations

        \item Assume you are reviewing a privacy policy, do you focus more on specific sections or general overview?

        Scale: Focus much more on specific sections (1) - Focus much more on general overview (5)

        %Scale: Focus on general overview, Slightly prefer detailed content, Neutral, Prefer detailed content, Strongly prefer detailed content
        
    \end{itemize}
\item Computer Self-Efficacy:
    \begin{itemize}
        \item How confident are you in your ability to manage privacy settings on social media platforms? (Scale of 1-10)

        Polarity: 1 means `Not confident at all’ and 10 means ‘Extremely confident’
        
        % \item How comfortable are you with using technologies that protect your privacy, such as virtual private networks (VPNs) and encryption tools?
        %JED: there seems to be a second category of tools, to inspect your hygiene (i.e., it has been 60 days since you last changed password, are you annoyed or relieved?)

        % Polarity: 1 means ‘Not comfortable at all’ and 10 means ‘Very comfortable’
    \end{itemize}
\item Risk Aversion:
    \begin{itemize}
        \item How much do potential security threats influence your online behavior?

        Polarity: 1 means ‘Not influenced at all’ and 10 means ‘Extremely influenced’
        
        \item How often do you avoid using services that have unclear or complicated privacy policies? (Scale of 1-10)
        %JED: we might also want to incorporate the idea of the pp being "invasive" or similar

        Polarity: 1 means ‘Never avoid’ and 10 means ‘Always avoid’
    \end{itemize}
\item Psychological Perceptions:
    \begin{itemize}
        \item How important is it for you to feel in control of your personal information online?
        %JED: run this by Dunni, this strikes me as very related to Need for Agency...something

        Polarity: 1 means ‘Not important at all’ and 10 means ‘Extremely important’
        
        \item How frequently do you worry about your personal information being misused by companies? (Scale of 1-10)

        Polarity: 1 means ‘Never’ and 10 means ‘Frequently’
    \end{itemize}
\item Decision-Making:
    \begin{itemize}
        \item How much do privacy concerns influence your decision to use or not use an online service? (Scale of 1-10)
        %JED: based on reading and RA1, we might prefer just collecting a qualitative data, so after How much does it influence... What do you do differently?
        % possible alternative. How often have you based your decion to use or not use an online service on privacy concerns? Never to frequently

        Polarity: 1 means ‘No influence’ and 10 means ‘Extremely influential’
        
        \item How likely are you to read reviews or seek expert opinions about a service’s privacy practices before using it?

        Polarity: 1 means ‘Very unlikely’ and 10 means ‘Very likely’
    \end{itemize}
\item Cognitive Style:
    \begin{itemize}
        \item How much do you rely on logical reasoning versus intuition when assessing privacy risks?
        scale : not much to a lot
        %\item How detailed do you prefer the explanations of privacy policies to be? (Scale of 1-10)
        %JED I think this is duplicative
    \end{itemize}
\item Behavioral Tendencies:
    \begin{itemize}
        \item How proactive are you in updating your privacy settings regularly?

        Polarity: 1 means ‘Never proactive’ and 10 means ‘Always proactive’

        (If 5, Scale: Never proactive, Rarely proactive, Sometimes proactive, Often proactive, Always proactive)
        
        \item How likely are you to participate in privacy awareness programs or workshops? (Scale of 1-10)

        Polarity: 1 means ‘Very unlikely’ and 10 means ‘Very likely’
        %JED: we may want to either add an option to say "i do that" or give them a qualitative response option too.
    \end{itemize}
\item Trust in Technology:
    \begin{itemize}

        \item How comfortable are you with sharing personal information with online services you use regularly?

        Polarity: 1 means ‘Not comfortable at all’ and 10 means ‘Very comfortable’
    \end{itemize}
\item Experience with Privacy Breaches:
    \begin{itemize}
        \item Have you ever experienced a privacy breach? If so, how did it affect your trust in online services? 
        \\
        List: Account Hacked, Data Breach, Received recommendations without opting-in, Received personalized ads without opting-in, Failed to obtain a refund, Observed unexpected charges, Account suspended/terminated, Misunderstood your rights or responsibilities, Data Misused in some other way
        Scale: Yes/No        
        %JED: answer is yes, and they are lying if they say otherwise

        % \item On a scale of 1-10, how vigilant are you about monitoring your online accounts for suspicious activities?

        % Polarity: 1 means ‘Not vigilant at all’ and 10 means ‘Extremely vigilant’
        %JED: we should take three questions (proactive, monitoring, think about) and reduce them down to 1-2
    \end{itemize}
\end{enumerate}

\section{Final List}

\begin{enumerate}
    \item What is your age range? (according to US Census)
    \begin{itemize}
        \item 18-24
        \item 25-34
        \item 35-44
        \item 45-54
        \item 55-64
        \item 65-74
        \item 75 and above
    \end{itemize}

    \item What is your occupation? (based on US Census)

    \begin{itemize}
        \item Management
            \begin{enumerate}
                \item Managers (all types, like sales, marketing, operations)
            \end{enumerate}
        \item Business and Finance
            \begin{enumerate}
                \item Accountants, financial analysts, HR specialists
            \end{enumerate}
        \item Computer and Mathematical
            \begin{enumerate}
                \item • Software developers, IT support, data analysts
            \end{enumerate}
        \item Architecture and Engineering
            \begin{enumerate}
                \item Engineers (civil, mechanical, electrical), architects
            \end{enumerate}
        \item Science
            \begin{enumerate}
                \item Biologists, chemists, environmental scientists
            \end{enumerate}
        \item Community and Social Services
            \begin{enumerate}
                \item Social workers, counselors, religious workers
            \end{enumerate}
        \item Legal 
            \begin{enumerate}
                \item Lawyers, paralegals, legal assistants
            \end{enumerate}
        \item Education
            \begin{enumerate}
                \item Teachers, professors, librarians
            \end{enumerate}
        \item Arts and Media
            \begin{enumerate}
                \item Artists, writers, designers, journalists
            \end{enumerate}
        \item Healthcare Practitioners and Technicians
            \begin{enumerate}
                \item Doctors, nurses, pharmacists, lab technicians
            \end{enumerate}
        \item Protective Services
            \begin{enumerate}
                \item Police officers, firefighters, security guards
            \end{enumerate}
        \item Food Preparation and Serving
            \begin{enumerate}
                \item Chefs, waiters, bartenders
            \end{enumerate}
        \item Office and Administrative Support
            \begin{enumerate}
                \item Secretaries, office clerks, customer service representatives
            \end{enumerate}
        \item Farming, Fishing, and Forestry
            \begin{enumerate}
                \item Farmers, fishers, logging workers
            \end{enumerate}
        \item Construction and Extraction
            \begin{enumerate}
                \item Construction workers, electricians, plumbers
            \end{enumerate}
        \item Installation, Maintenance, and Repair
            \begin{enumerate}
                \item Mechanics, electricians, repair workers
            \end{enumerate}
        \item Transportation and Material Moving
            \begin{enumerate}
                \item Truck drivers, delivery drivers, warehouse workers
            \end{enumerate}
        \item Sales
            \begin{enumerate}
                \item Retail salespersons, real estate agents, sales representatives
            \end{enumerate}
    \end{itemize}

    \item  What is your nationality?

    \begin{itemize}
        \item United States
        \item Canada
        \item Mexico
        \item United Kingdom
        \item China
        \item India
        \item Phillipines
        \item Germany
        \item Argentina
        \item Brazil
        \item France
        \item Italy
        \item Spain
        \item If none of the above, self-describe TEXTBOX
    \end{itemize}

    \item How motivated are you to read privacy policies before using an online service to make sure your information is safe?	

    Polarity: 1 means ‘Not motivated at all’ and 10 means ‘Extremely motivated’

    \item How likely are you to invest time in understanding privacy policies to avoid potential privacy issues?
        
    Polarity: 1 means ‘Very unlikely’ and 10 means ‘Very likely’

    \item Assume you are reviewing a privacy policy, do you focus more on specific sections or a general overview?

    Scale: Focus much more on specific sections (1) - Focus much more on general overview (5)

    \item How confident are you in your ability to manage privacy settings on social media platforms?

    Polarity: 1 means `Not confident at all’ and 10 means ‘Extremely confident’
        
    \item How comfortable are you with using technologies that protect your privacy, such as virtual private networks (VPNs), or inspect your privacy hygiene, such as Ghostery?

    Polarity: 1 means ‘Not comfortable at all’ and 10 means ‘Very comfortable’

    \item How important is it for you to feel in control of your personal information online?

    Polarity: 1 means ‘Not important at all’ and 10 means ‘Extremely important’

    \item How proactive are you in updating your privacy settings regularly?

    Polarity: 1 means ‘Never proactive’ and 10 means ‘Always proactive’

    \item How comfortable are you with sharing personal information with online services you use regularly?

    Polarity: 1 means ‘Not comfortable at all’ and 10 means ‘Very comfortable’

    \item Despite the risks, how often do you accept terms and conditions before reading them?

    Polarity: 1 means ‘Never’ and 5 means ‘Always’

    \item How likely are you to take action (e.g., change settings, stop using a service) if you find a privacy policy concerning?
    
    Polarity: 1 means ‘Very unlikely’ and 10 means ‘Very likely’

    %JED: could imagine asking a qualitative question "what action would you take" (I don't feel strongly on this one)

    \item Have you ever had any of the following negative experiences due to not understanding or not reading a privacy policy?
    
    (E.g., Account getting hacked, Data used elsewhere, Account discontinued, no refund, etc.

    List: Account Hacked, 
    Data Breach,
    Received recommendations without opting-in,
    Received personalized ads without opting-in,
    Failed to obtain a refund,
    Observed unexpected charges,
    Account suspended/terminated,
    Misunderstood your rights or responsibilities,
    Data Misused in some other way
    
    Scale: Yes/No

    % Validate with the team 
    
    \item Suppose educational resources or tools were available to help you better understand privacy policies, how much would you be interested to learn more about such resources?
    % Would you be interested in educational resources or tools to help you better understand privacy policies?

    Polarity: 1 means ‘Not interested at all’ and 10 means ‘Extremely interested’

\end{enumerate}
